# Supplementary material for: Tor's Been KIST: A Case Study of Transitioning Tor Research to Practice
Source: arXiv:1709.01044 source file (2017-09-04)
Supplement: Supplementary file 1 [file appendix.tex]

\appendix
%\appendixpage

\section*{Appendix}

\begin{figure*}[h!]
\centering
\subfloat[All, Varying Load]{\label{fig:perf:load:ttfb-6hop}{\includegraphics[width=0.30\textwidth]{load-ttfb-6hop.pdf}}}
\subfloat[Web, Varying Load]{\label{fig:perf:load:ttlb-web-6hop}{\includegraphics[width=0.30\textwidth]{load-ttlb-web-6hop.pdf}}}
\subfloat[Bulk, Varying Load]{\label{fig:perf:load:ttlb-bulk-6hop}{\includegraphics[width=0.30\textwidth]{load-ttlb-bulk-6hop.pdf}}}
\\
\subfloat[All, Varying Loss]{\label{fig:perf:loss:ttfb-6hop}{\includegraphics[width=0.30\textwidth]{loss-ttfb-6hop.pdf}}}
\subfloat[Web, Varying Loss]{\label{fig:perf:loss:ttlb-web-6hop}{\includegraphics[width=0.30\textwidth]{loss-ttlb-web-6hop.pdf}}}
\subfloat[Bulk, Varying Loss]{\label{fig:perf:loss:ttlb-bulk-6hop}{\includegraphics[width=0.30\textwidth]{loss-ttlb-bulk-6hop.pdf}}}
\caption{Client performance shown as time to receive the first and last byte of each download for clients using long 6-hop onion service circuits. Performance is shown across our varying traffic load and packet loss models described in \S\ref{sec:simeval:net}.}
\label{fig:perf:6hop}
\end{figure*}
